# Supplementary material for: On eigenvalues of the Schr\"odinger operator with an even complex-valued polynomial potential
Source: arXiv:1104.0593 source file (2011-04-04)
Supplement: Supplementary file 7 [file si_action_case3_before.tex]

\documentclass[a4paper,11pt,dvips]{paper}
\usepackage[all]{xy}
\xyoption{ps}
\xyoption{dvips}

\input{../sections/definitions.tex}

\begin{document}
\pagestyle{empty}

\xymatrix @-1pc {
\cdot & \cdots & \cdot & & \cdot & \cdots & \cdot & & \cdot & \cdots & \cdot & & \cdot & \cdots & \cdot\\
 &\bullet \ar@{..}[l]  \ar@{--}[ul] \ar@{--}[u] \ar@{--}[ur] & & & 
 &\bullet \ar@{--}[ul] \ar@{--}[u] \ar@{--}[ur] \ar@{->}[llll]^{\edge_{j}} & & &
 &\bullet_\junc \ar@{--}[ul] \ar@{--}[u] \ar@{--}[ur] \ar@{->}[llll]^{\edge_{j}} & & &
 &\bullet \ar@{..}[r] \ar@{--}[ul] \ar@{--}[u] \ar@{--}[ur] \ar@{->}[llll]^{\edge_{j_+}} & & & \\
\\
&&&& &w_j  & & &  \bullet \ar@{->}[uur]^{\edge_{j}} &  & \bullet \ar@{<-}[uul]_{\edge_{j_+}} & & w_{j_+} & & \\
&&&& & & & \ar@{..}[ur] &  & w_{j+1}=0  & & \ar@{..}[ul] & & \\
}
\end{document}
