# Supplementary material for: On eigenvalues of the Schr\"odinger operator with an even complex-valued polynomial potential
Source: arXiv:1104.0593 source file (2011-04-04)
Supplement: Supplementary file 9 [file si_action_case3_middle.tex]

\documentclass[a4paper,11pt,dvips]{paper}
\usepackage[all]{xy}
\xyoption{ps}
\xyoption{dvips}

\input{../sections/definitions.tex}

\begin{document}
\pagestyle{empty}

\xymatrix @-1pc {
\cdot & \cdots & \cdot & & \cdot & \cdots & \cdot & & \cdot & \cdots & \cdot & & \cdot & \cdots & \cdot\\
 &\bullet \ar@{..}[l]  \ar@{--}[ul] \ar@{--}[u] \ar@{--}[ur] & & & 
 &\bullet \ar@{--}[ul] \ar@{--}[u] \ar@{--}[ur] \ar@{->}[llll]^{\edge_{j_+}} & & &
 &\bullet_\junc \ar@{--}[ul] \ar@{--}[u] \ar@{--}[ur] & & &
 &\bullet \ar@{..}[r] \ar@{--}[ul] \ar@{--}[u] \ar@{--}[ur] \ar@{->}[llll]^{\edge_{j}} & & & \\
&& &     & & & & \bullet  \ar@{->}[ull]^{\edge_{j_+}}  \ar@{<-}[urr]_{\edge_{j}} &&&&&&&&\\
\\
&& &w_{j_+}  & & &  \bullet \ar@{->}[uur]^{\edge_{j_+}} &  & \bullet \ar@{<-}[uul]_{\edge_{j}} & & w_{j} & & \\
&& & & & \ar@{..}[ur] &  & w_{j+1}=0  & & \ar@{..}[ul] & & \\
}
\end{document}
